# Supplementary material for: InsTALL: Context-aware Instructional Task Assistance with Multi-modal Large Language Models
Source: arXiv:2501.12231 source file (2025-01-21)
Supplement: Supplementary file 1 [file supp.tex]

\twocolumn[{
\renewcommand\twocolumn[1][]{#1}%
\begin{center}
\maketitlesupplementary
\centering
\captionsetup{type=figure}
\includegraphics[width=\textwidth]{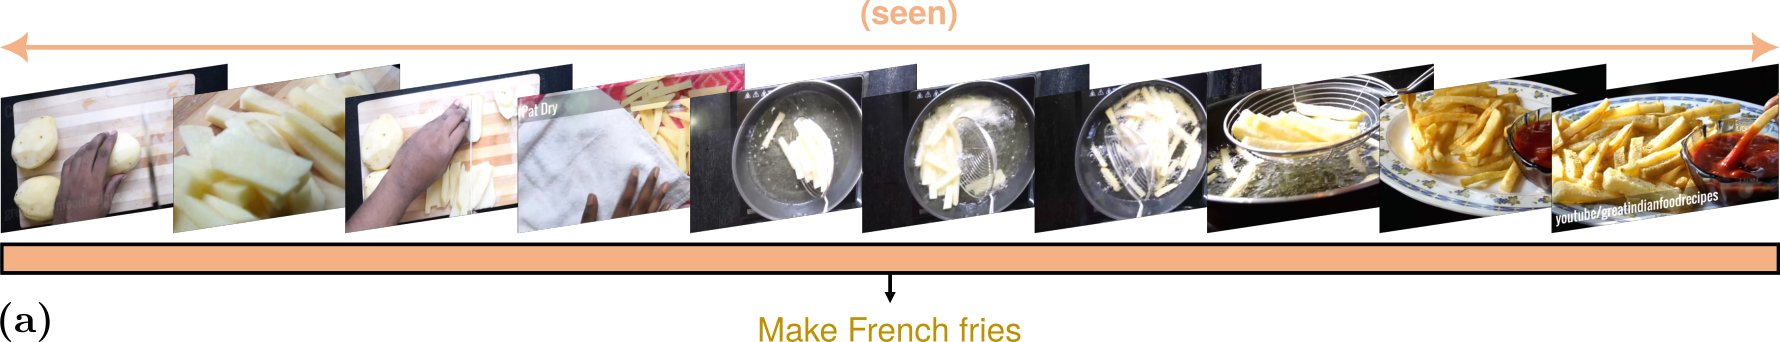}
\vspace{0.5\baselineskip}
\includegraphics[width=\textwidth]{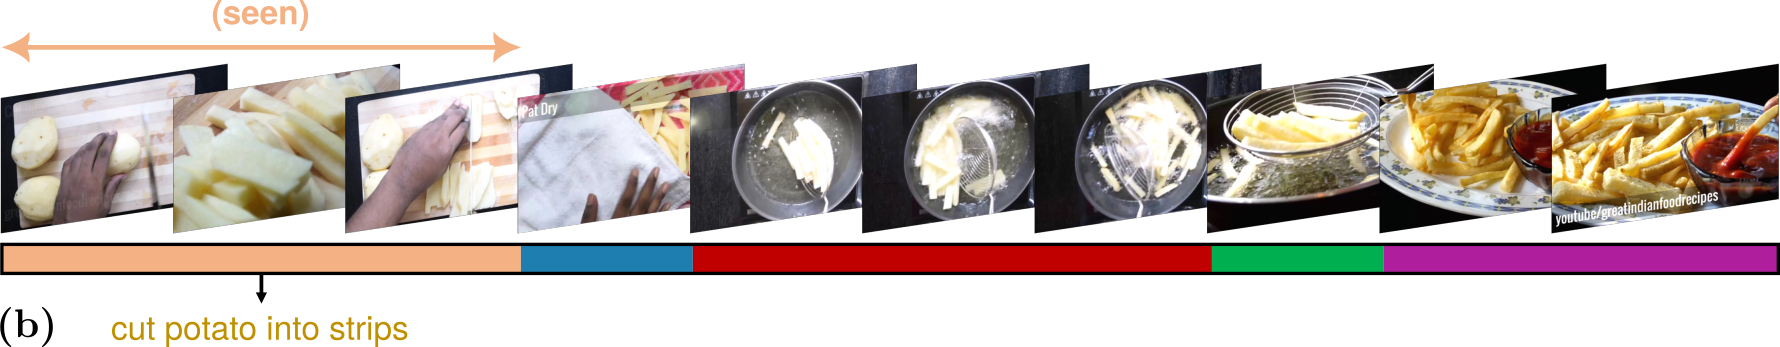}
\vspace{0.5\baselineskip}
\includegraphics[width=\textwidth]{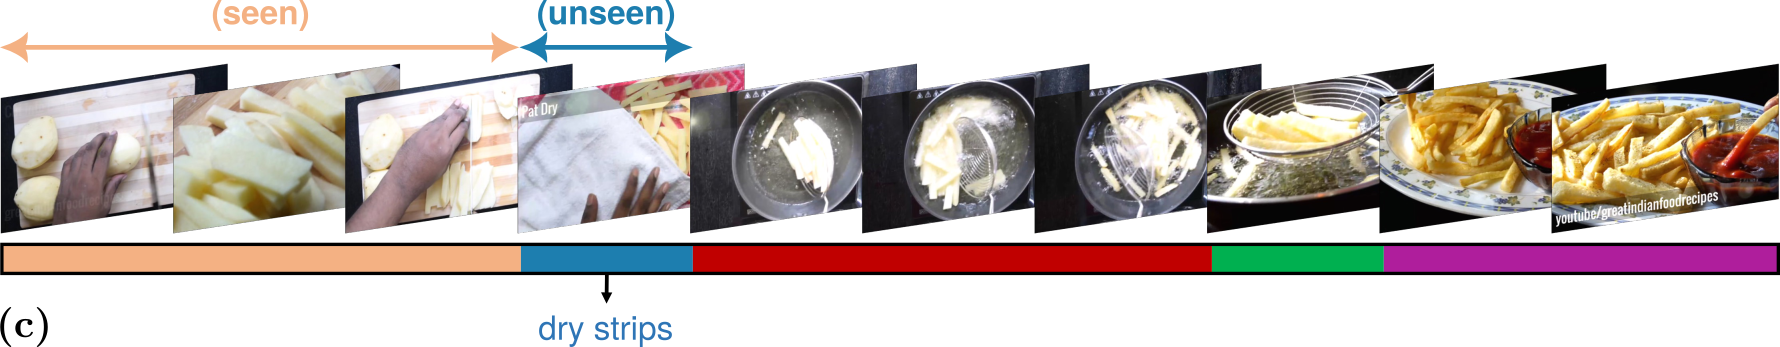}
\vspace{0.5\baselineskip}
\includegraphics[width=\textwidth]{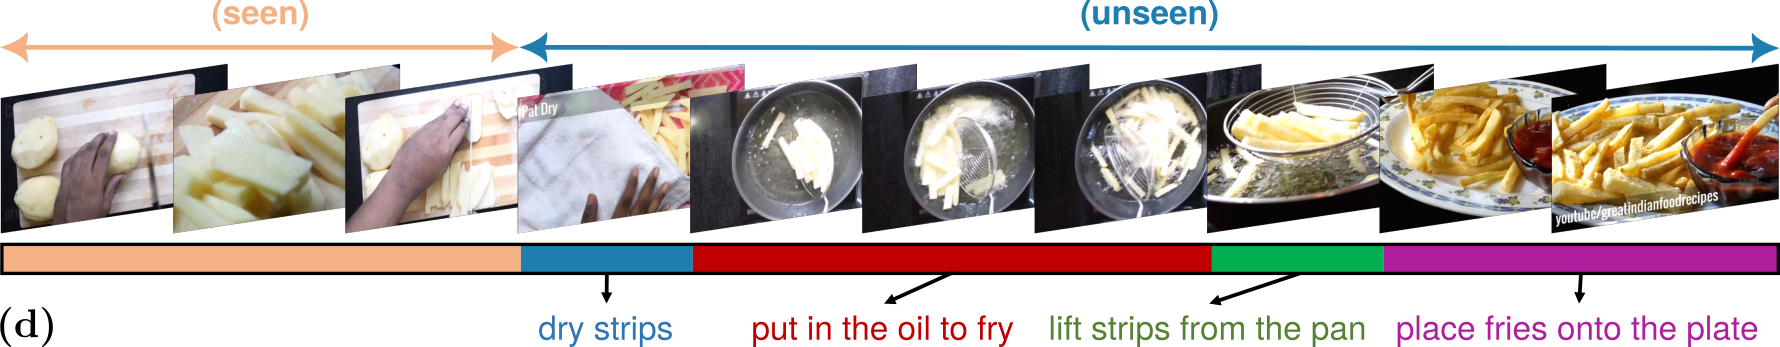}
\captionof{figure}{Visualization of the introduced tasks, including (a) Task Recognition, (b) Action Recognition, (c) Action Prediction, and (d) Plan Prediction. The differences in task definitions mainly are the portions in seen and unseen video clips as clearly stated in equations.}
\label{fig:supp_teaser}
\end{center}
}]

\section{Task Visualization}

We visualize the process of predicting the introduced tasks in Fig.~\ref{fig:supp_teaser} and provide a tiny set of those tasks in \texttt{tiny.zip}. For convenience, we include the definition of these tasks as below.

\noindent \textbf{Task Recognition (TR).} Given a video snippet $\mathbf{V}$ (Fig.~\ref{fig:supp_teaser}a) and a task prompt $\mathbf{Q}_{\texttt{TR}}$, we seek to identify the task being performed by minimizing the following objective:
\begin{equation}
\min \mathbb{E}_{\mathbf{V}, Y} \bigg[-\sum_{i=1}^{n} Y_i\log\Big(\mathbbm{1}_{Y}\big(p(\mathbf{T} | \mathbf{V}, \mathbf{Q}_{\texttt{TR}})\big)_i\Big)\bigg]
\label{eq:tr}
\end{equation}
where $\mathbf{T}$ is the text response from the MLLM. As this is a classification task, we expect a one-hot mapping that maps the response to the set of task categories $Y$, \ie, denoted as $\mathbbm{1}_{Y}(\cdot)$, and $n = |Y|$.

\noindent \textbf{Action Recognition (AR).} Given a clipped video $\mathbf{v}_{t}$ and a task prompt $\mathbf{Q}_{\texttt{AR}}$ (Fig.~\ref{fig:supp_teaser}b), we seek to identify the action being performed in it by minimizing the following objective:
\begin{equation}
\min \mathbb{E}_{\keyword{\mathbf{v}_{t}}, y} \bigg[-\sum_{i=1}^{m} y_i\log\Big(\mathbbm{1}_{y}\big(p(\mathbf{a}_{t} | \keyword{\mathbf{v}_{t}}, \mathbf{Q}_{\texttt{AR}})\big)_i\Big)\bigg]
\label{eq:ar}
\end{equation}
where $\mathbf{a}_{t}$ is the answer and $y_i$ is the action/step annotation for clip $\mathbf{v}_{t} (\in \mathbf{V})$, and $m = |y|$.

\noindent \textbf{Action Prediction (AP).}  Given the task prompt $\mathbf{Q}_{\texttt{AP}}$, a video upto a particular point $\mathbf{v}_{<t}$ (Fig.~\ref{fig:supp_teaser}c), we learn to predict the next likely step $\mathbf{a}_{t}$ by minimizing the objective below:
\begin{equation}
\min \mathbb{E}_{\keyword{\mathbf{v}_{< t}}, y} \bigg[-\sum_{i=1}^{m} y_i\log\Big(\mathbbm{1}_{y}\big(p(\mathbf{a}_{t} | \keyword{\mathbf{v}_{< t}}, \mathbf{Q}_{\texttt{AP}})\big)_i\Big)\bigg]
\label{eq:ap}
\end{equation}

\noindent \textbf{Plan Prediction (PP).} Given the task prompt $\mathbf{Q}_{\texttt{PP}}$, a video upto a particular point $\mathbf{v}_{<t}$ (Fig.~\ref{fig:supp_teaser}d), we seek to predict an ordered list of actions $\mathbf{a}_{\geq t}$ by minimizing the multiple-class mapping function $\mathbb{T}_{y}(\cdot)$:
\begin{equation}
\min \mathbb{E}_{\keyword{\mathbf{v}_{< t}}, y} \bigg[-\sum_{i=1}^{m} y_i\log\Big(\keyword{\mathbb{T}_{y}}\big(p(\keyword{\mathbf{a}_{\geq t}} | \keyword{\mathbf{v}_{< t}}, \mathbf{Q}_{\texttt{PP}})\big)_i\Big)\bigg]
\label{eq:pp}
\end{equation}
where the number of procedural steps in $|\keyword{\mathbf{a}_{\geq t}}| > |\mathbf{a}_t| = 1$.

\begin{figure*}[!t]
 \centering
 \includegraphics[width=0.95\textwidth]{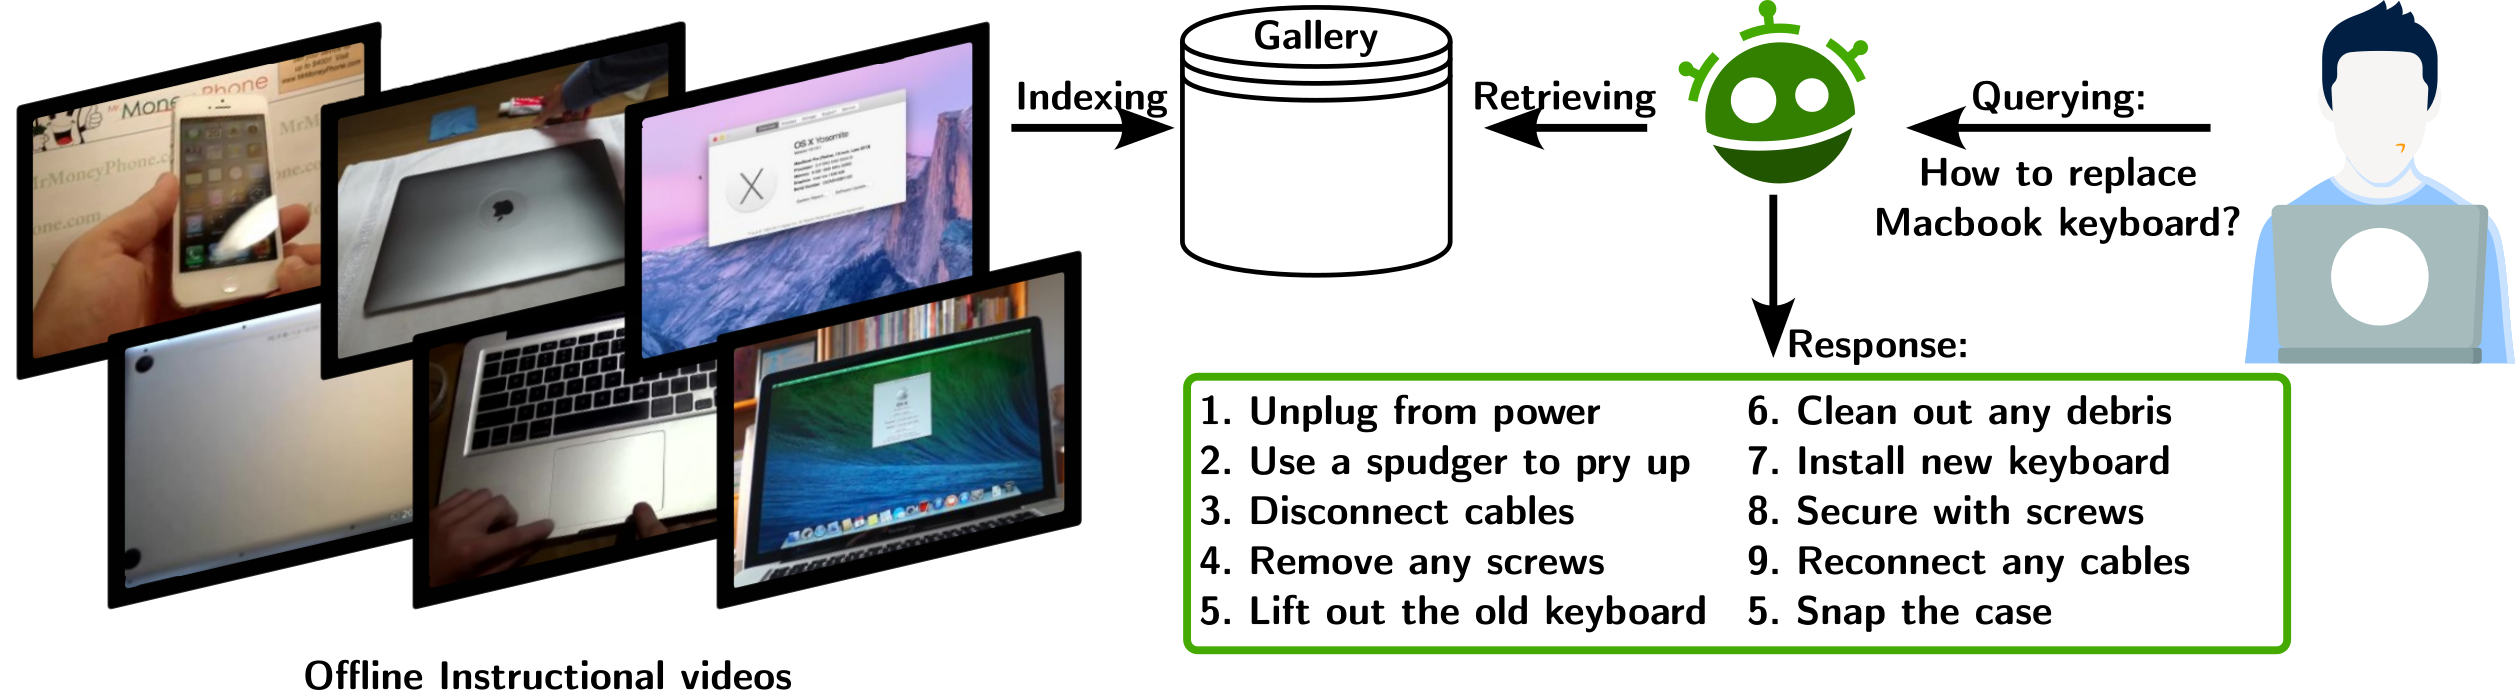}
 \caption{Visualization of the VectorRAG approach.}
 \label{fig:supp_vectorrag}
\end{figure*}

\section{VectorRAG Approach}

The VectorRAG design focuses on identifying the correct video step corresponding to a given text query from a collection of videos in a test set. It achieves this by adapting state-of-the-art video retrieval techniques that embed both text and video content into a shared feature space using an encoder, denoted as $\psi$ and $\phi$. This shared space allows for direct comparison between the embeddings of videos and the textual query.

The process involves finding the video with the embedding most similar to the reference derived from the query. Mathematically, this is expressed as selecting the video $\mathbf{V}$ that maximizes the cosine similarity between its embedding and the query embedding. The similarity measure is represented as:
\begin{equation}
\big\langle \psi(\mathbf{V}), \phi(\mathbf{A}) \big\rangle
\end{equation}

It ensures that the selected video aligns closely with the semantic meaning of the query as illustrated in Fig.~\ref{fig:supp_vectorrag}.

One of the methods used is CLIP~\cite{radford2021learning}, a state-of-the-art vision-language model that has been extensively applied to multi-modal tasks. CLIP operates on short video clips as input, and to represent an entire video, it computes the average of the embeddings of all the short-term features. This approach effectively condenses the temporal information within videos into a robust feature representation.

The performance of the VectorRAG approach is evaluated using standard retrieval metrics, including precision, recall, and F1 score. These metrics, as adopted from prior work on multi-modal retrieval, provide a comprehensive assessment of how well the method identifies relevant video steps based on the input text queries.
